# Supplementary material for: Two-dimensional anisotropic Dirac materials PtN4C2 and Pt2N8C6 with quantum spin and valley Hall effects
Source: arXiv:2207.03703 source file (2022-07-08)
Supplement: Supplementary file 1 [file Supplementary_Materials.pdf]

# Two-dimensional anisotropic Dirac materials $\text{PtN}_4\text{C}_2$ and $\text{Pt}_2\text{N}_8\text{C}_6$ with quantum spin and valley Hall effects

Jingping Dong<sup>1,\*</sup>, Chuhan Wang<sup>1,\*</sup>, Xinlei Zhao<sup>1</sup>, Miao Gao<sup>2</sup>, Xun-Wang Yan<sup>3,†</sup>, Fengjie Ma<sup>1,‡</sup> and Zhong-Yi Lu<sup>4</sup>

<sup>1</sup>The Center for Advanced Quantum Studies and Department of Physics,  
Beijing Normal University, Beijing 100875, China

<sup>2</sup>Department of Physics, School of Physical Science and Technology, Ningbo University, Zhejiang 315211, China

<sup>3</sup>College of Physics and Engineering, Qufu Normal University, Shandong 273165, China and

<sup>4</sup>Department of Physics, Renmin University of China, Beijing 100872, China

## A. The phonon spectrum of $\text{Pt}_2\text{N}_8\text{C}_6$

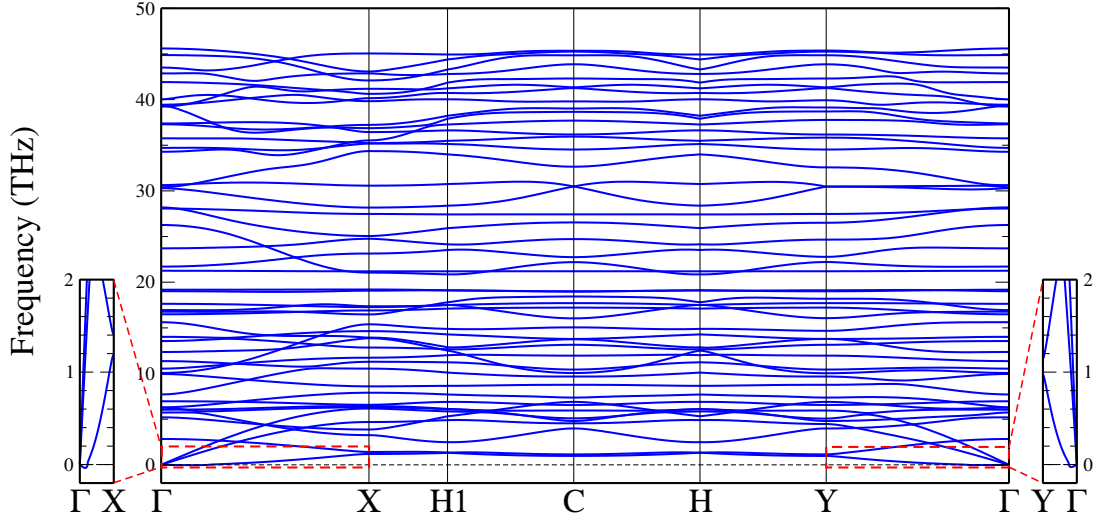

FIG. S1: Phonon spectrum of  $\text{Pt}_2\text{N}_8\text{C}_6$ .

Figure S1 shows the phonon spectrum of  $\text{Pt}_2\text{N}_8\text{C}_6$ . There is no considerable imaginary frequency to appear in the entire Brillouin zone, indicating that the  $\text{Pt}_2\text{N}_8\text{C}_6$  monolayer is dynamically stable. Note that there are two tiny spoon-shaped pockets near the  $\Gamma$  point along  $\Gamma$ -X and  $\Gamma$ -Y paths as shown in the zoomed-in graphs, which are due to the difficulty of achieving numerical convergence for the flexural phonon branch. It is a common issue in the first-principles electronic structure calculations on 2D materials and does not imply instability [1, 2].

## B. The band structural and electronic properties of $\text{Pt}_2\text{N}_8\text{C}_6$

Figure S2(a) shows the calculated electronic band structure of  $\text{Pt}_2\text{N}_8\text{C}_6$ . Similar to  $\text{PtN}_4\text{C}_2$ ,  $\text{Pt}_2\text{N}_8\text{C}_6$  is also a perfect Dirac semi-metal, with a linearly dispersive Dirac node presented at a general k-point in the high symmetry path  $Y$ - $\Gamma$ . By projecting the band structures onto different atomic orbitals, the Dirac node is found to mainly consist of N- $p$ , C- $p$ , and Pt- $d$  states. More specifically, the C- $p_z$  and N- $p_z$  form a  $\pi$  network together with the Pt  $d_{xz}$  and  $d_{yz}$  orbitals in the vicinity of the Fermi level, as shown in Fig. S2(b). Figures S2(c) and S2(d) give the zoomed-in view of the area around the Dirac point with orbital projections and the corresponding three-dimensional energy dispersion of bands without spin-orbit coupling.

\*These authors contributed equally to this work.

<sup>†</sup>Electronic address: [yanxunwang@163.com](mailto:yanxunwang@163.com)

<sup>‡</sup>Electronic address: [fengjie.ma@bnu.edu.cn](mailto:fengjie.ma@bnu.edu.cn)

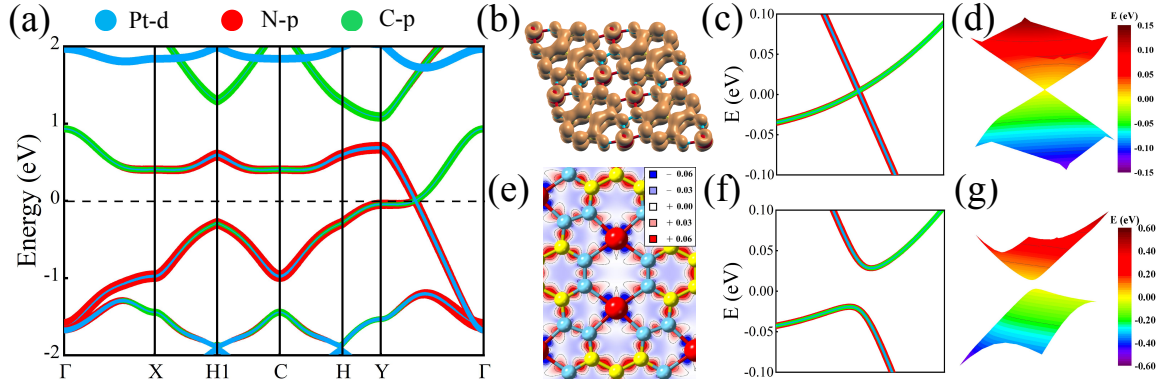

FIG. S2: (a) Orbital-resolved band structure of monolayer  $\text{Pt}_2\text{N}_8\text{C}_6$  without spin-orbit coupling. The black dashed line represents the Fermi level. (b) The charge density distributions from the wavefunctions of the lowest conduction and highest valence bands of  $\text{Pt}_2\text{N}_8\text{C}_6$  at the Dirac point. A  $\pi$  network is formed by the C- $p_z$  and N- $p_z$  together with the Pt  $d_{xz}$  and  $d_{yz}$  orbitals. Here the isovalue is set to 0.0022 e/bohr<sup>3</sup>. (c) and (d) give the zoomed-in view of the area around the Dirac point with orbital projections and the corresponding three-dimensional energy dispersion of bands without spin-orbit coupling. (e) The distribution of differential charge density. The red and blue in the isosurface views represent the accumulation and depletion of electrons in units of e/bohr<sup>3</sup>, respectively. (f) and (g) show the zoomed-in view of the area around the Dirac point with orbital projections and the corresponding three-dimensional energy dispersion of bands with spin-orbit coupling.

In Fig. S2(e), we further calculate the differential charge density of  $\text{Pt}_2\text{N}_8\text{C}_6$  to illustrate the internal bonding conditions and charge transfers. The red/blue color represents the increase/decrease of charge density, indicating that covalent bonds are formed between the C-N, N-N, and C-C atoms and ionic bonds are formed between Pt and N atoms. After introducing spin-orbit coupling, an energy gap,  $\sim 40$  meV, is opened at the Dirac point, turning the linear band dispersions into quadratic ones, as shown in Fig. S2(f). Figure S2(g) illustrates the three-dimensional energy dispersion of highest valence and lowest conduction bands of  $\text{Pt}_2\text{N}_8\text{C}_6$  near the Dirac point with spin-orbit coupling.

### C. Topological properties of $\text{Pt}_2\text{N}_8\text{C}_6$

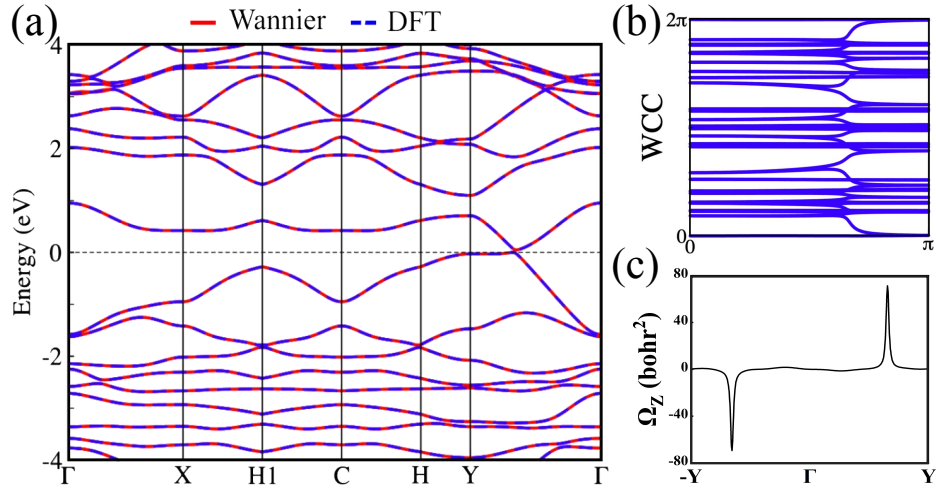

FIG. S3: (a) The comparison of the band structure of  $\text{Pt}_2\text{N}_8\text{C}_6$  from the Wannier tight-binding Hamiltonian (red solid lines) and the DFT calculations (blue dashed lines). Spin-orbit coupling is included. (b) The evolution of Wannier charge center (WCC) curves in half Brillouin zone to calculate the  $\mathbb{Z}_2$  invariant. (c) The Berry curvature along high-symmetry  $-Y-\Gamma-Y$  path in the Brillouin zone.

As shown in Fig. S3(a), the band structure constructed by the means of maximally localized wannier functions agrees very well with the results from the DFT calculations, in which Pt- $s, p, d$ , N- $s, p$ , and C- $s, p$  orbitals are adopted as the projection orbitals. In Fig. S3(b), it is clear from the figure that the Wannier charge center evolution curves cut an arbitrary horizontal reference line odd times, indicating a value of  $\mathbb{Z}_2 = 1$ . Thus the gapped  $\text{Pt}_2\text{N}_8\text{C}_6$  with spin-orbit coupling is a two-dimensional  $\mathbb{Z}_2$  topological insulator. Furthermore, from Fig. S3(c), the distribution of Berry curvature shows that the Berry phases around the two Dirac points within the Brillouin zone are opposite, as determined by the time-reversal symmetry, indicating that  $\text{Pt}_2\text{N}_8\text{C}_6$  is also a quantum valley Hall insulator.

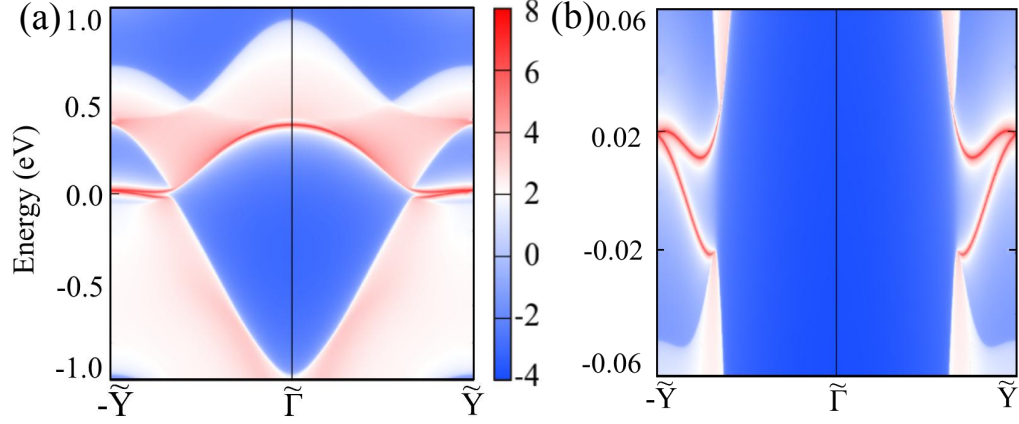

FIG. S4: (a) The helical edge and bulk band structure of  $\text{Pt}_2\text{N}_8\text{C}_6$  projected along the (100) direction. (b) Zoomed-in view of the area in a range of -0.06 to 0.06 eV.

Figure S4(a) shows the helical edge states of  $\text{Pt}_2\text{N}_8\text{C}_6$  projected along the (100) direction. Topological nontrivial edge states are visible, which across the bulk band gap and connect the bulk conduction and valence bands of  $\text{Pt}_2\text{N}_8\text{C}_6$  at the two projected Dirac points in the Brillouin zone along the high-symmetry line  $-\tilde{Y}-\tilde{\Gamma}-\tilde{Y}$ . Figure S4(b) gives the zoomed-in view of the area in a range of -0.06 to 0.06 eV.

- 
- [1] V. Zólyomi, N. D. Drummond, and V. I. Fal'ko, Physical Review B **89**, 205416 (2014).
  - [2] H. D. Tran, M. Amsler, S. Botti, M. A. L. Marques, and S. Goedecker, The Journal of Chemical Physics **140**, 124708 (2014).
